# Supplementary material for: Classification of Edge-dependent Labels of Nodes in Hypergraphs
Source: arXiv:2306.03032 source file (2023-06-05)
Supplement: Supplementary file 1 [file 090appendix.tex]

\begin{table*}[t]
    \vspace{-3mm}
	\begin{center}
		\caption{\label{tab:datasets} Dataset Statistics.}
		%\vspace{-1mm}
		\scalebox{0.8}{
		    \begin{tabular}{c c| c  c  c  c  c | c c c c c}
				\toprule
				\multicolumn{2}{c|}{Dataset} & \bigcell{c}{Num.\\Nodes} & \bigcell{c}{Num.\\Hyperedges} & \bigcell{c}{Max.\\Node Deg.} & \bigcell{c}{Max.\\Hyperedge Sz.} & \bigcell{c}{Num.\\NonZero} & \bigcell{c}{Num.\\Class 0} & \bigcell{c}{Num.\\Class 1} & \bigcell{c}{Num.\\Class 2} & \bigcell{c}{Corr.\\w/ Centrality} & \bigcell{c}{Avg.\\Entropy}\\ 
				\midrule
				\multirow{6}{*}{\shortstack{Edge-Dependent\\NodeLabel\\Prediction}} & Coauth-DBLP & 108,484 & 91,266 & 236 & 36 & .000,032 & 91,266 & 138,479 & 91,266 & 0.19 & 0.13\\ 
				& Coauth-AMiner & 1,712,433 & 2,037,605 & 752 & 115 & .000,001 & 2,037,605 & 1,652,332 & 1,503,061 & 0.24 & 0.13\\
				& Email-Enron & 21,251 & 101,124 & 18,168 & 948 & .000,552 & 635,268 & 450,129 & 101,124 & 0.10 & 0.28\\
				& Email-Eu & 986 & 209,508 & 8,659 & 59 & .002,623 & 209,508 & 332,334 & - & 0.24 & 0.48 \\
				& Stack-Biology & 15,490 & 26,823 & 1,318 & 12 & .000,135 & 26,290 & 18,444 & 11,523 & 0.29 & 0.10\\
				& Stack-Physics & 80,936 & 200,811 & 6,332 & 48 & .000,030 & 194,575 & 201,121 & 84,113 & 0.30 & 0.12\\
				\midrule
				\multirow{3}{*}{\shortstack{DownStream\\Task}} & Ranking-Halo & 5,507 & 31,028 & 505 & 12 & .001,120 & \multicolumn{3}{c}{Continuous value of scores in (0,1)} & 0.03\\
				& Return-Synthetic & 6,000 & 9,675 & 10 & 13 & .000,575 & 3,406 & 19,918 & 10,082 & 0.01\\
				& Clustering-DBLP & 2,123 & 1,000 & 22 & 25 & .001,829 & 997 & 1,885 & 1,000 & 0.13\\
				\bottomrule
			\end{tabular}}
	\end{center}
	\vspace{-4mm}
\end{table*}

\begin{table*}[t]
    \begin{center}
        \caption{\label{tab:pe_ablation} Comparison of Positional Encoding Schemes.}
        \scalebox{0.8}{
            \begin{tabular}{c c | c c c c c c c||c c c}
            \toprule
            \multicolumn{2}{c|}{\multirow{2}{*}{Dataset}} & & \multicolumn{5}{c}{Positional Encodings} &&& \multicolumn{2}{c}{\PE} \\
            \cline{4-8} \cline{11-12}
            && w/o PE & GraphIT/DK & GraphIT/PRWK & Shaw/DK & Shaw/PRWK & WholeOrderPE &&& w/o Inducing Points & w/ Inducing Points  \\ 
            \midrule
            \multirow{2}{*}{\shortstack{Stack\\Biology}} & MicroF1 & 0.727 $\pm$ 0.005 & 0.718 $\pm$ 0.005 & 0.712 $\pm$ 0.003 & 0.733 $\pm$ 0.003 & 0.571 $\pm$ 0.061  & 0.723 $\pm$ 0.002 &&& 0.736 $\pm$ 0.003 & \textbf{0.737} $\pm$ 0.004 \\
            & MacroF1 & 0.664 $\pm$ 0.005 & 0.648 $\pm$ 0.004 & 0.646 $\pm$ 0.004 & 0.676 $\pm$ 0.005 & 0.468 $\pm$ 0.012 & 0.661 $\pm$ 0.003 &&& \textbf{0.679} $\pm$ 0.005 & 0.678 $\pm$ 0.005 \\
            \bottomrule
        \end{tabular}}
    \end{center}
	\vspace{-4mm}
\end{table*}

\begin{table*}[t]
    \begin{center}
        \caption{\label{tab:ablation2} Comparison of Architectures for Aggregation of Hyperedge Embeddings.}
        \scalebox{0.82}{
            \begin{tabular}{c c |c c c c c c|| c}
            \toprule
            \multicolumn{2}{c|}{\multirow{2}{*}{Dataset}} && & & \multicolumn{2}{c}{MSG. Passing from Hyperedge to Node} && \multirow{2}{*}{\method} \\
            \cline{6-7}
            & && HNHN & HAT & \method + HNHN & \method + HAT && \\ 
            \midrule
            \multirow{2}{*}{\shortstack{Stack\\Biology}} & MicroF1 && 0.636 $\pm$ 0.006 & 0.659 $\pm$ 0.006 & 0.669 $\pm$ 0.019 & 0.674 $\pm$ 0.004  && \textbf{0.738} $\pm$ 0.001\\
            & MacroF1 && 0.585 $\pm$ 0.001 & 0.604 $\pm$ 0.008 & 0.588 $\pm$ 0.047 & 0.620 $\pm$ 0.000  && \textbf{0.680} $\pm$ 0.003\\ 
            \bottomrule
        \end{tabular}}
    \end{center}
\end{table*}
% \begin{table}[t]
%     \begin{center}
%         \caption{\label{tab:ablation2} Ablation Study of Architecture for Aggregation at Nodes.}
%         \scalebox{0.6}{
%             \begin{tabular}{c | c c c c || c}
%             \toprule
%             & & & \multicolumn{2}{c}{MSG. Passing from Hyperedge to Node} & \multirow{2}{*}{\method} \\
%             \cline{4-5}
%             & HNHN & HAT & \method + HNHN & \method + HAT & \\ 
%             \midrule
%             MicroF1 & 0.636 $\pm$ 0.006 & 0.659 $\pm$ 0.006 & 0.669 $\pm$ 0.019 & 0.674 $\pm$ 0.004  & \textbf{0.738} $\pm$ 0.001\\
%             MacroF1 & 0.585 $\pm$ 0.001 & 0.604 $\pm$ 0.008 & 0.588 $\pm$ 0.047 & 0.620 $\pm$ 0.000  & \textbf{0.680} $\pm$ 0.003\\ 
%             \bottomrule
%         \end{tabular}}
%     \end{center}
% \end{table}

% \begin{table*}[h]
%     \begin{center}
%         \caption{\label{tab:ablation2} Ablation}
%         \scalebox{0.8}{
%             \begin{tabular}{c c |c c c c c c|c c c|| c}
%             \toprule
%             \multicolumn{2}{c|}{\multirow{2}{*}{Dataset}} && \multicolumn{4}{c}{MSG. Passing from Hyperedge to Node} &&& Aggregation && \multirow{2}{*}{\method} \\
%             \cline{4-7} \cline{10-10}
%             & && HNHN & HAT & \method + HNHN & \method + HAT &&& w/ PMA && \\ 
%             \midrule
%             \multirow{2}{*}{\shortstack{Stack\\Biology}} & MicroF1 && 0.636 $\pm$ 0.006 & 0.659 $\pm$ 0.006 & 0.669 $\pm$ 0.019 & 0.674 $\pm$ 0.004 &&& - && \textbf{0.738} $\pm$ 0.001\\
%             & MacroF1 && 0.585 $\pm$ 0.001 & 0.604 $\pm$ 0.008 & 0.588 $\pm$ 0.047 & 0.620 $\pm$ 0.000 &&& - && \textbf{0.680} $\pm$ 0.003\\ 
%             \bottomrule
%         \end{tabular}}
%     \end{center}
% \end{table*}

% \begin{table*}[ht]
%     \vspace{-3mm}
% 	\begin{center}
% 		\caption{\label{tab:datasets} Dataset Statistics.}
% 		%\vspace{-1mm}
% 		\scalebox{0.75}{
% 		    \begin{tabular}{c c| c  c  c  c  c | c c c | c c c c c}
% 				\toprule
% 				\multicolumn{2}{c|}{Dataset} & \bigcell{c}{Num.\\Nodes} & \bigcell{c}{Num.\\Hyperedges} & \bigcell{c}{MAX.\\Node Degree} & \bigcell{c}{MAX.\\Hyperedge Size} & \bigcell{c}{NNZ} & \bigcell{c}{Num.\\Class 0} & \bigcell{c}{Num.\\Class 1} & \bigcell{c}{Num.\\Class 2} & \bigcell{c}{Corr.\\Degree} & \bigcell{c}{Corr.\\Eigenvector} & \bigcell{c}{Corr.\\Pagerank} & \bigcell{c}{Corr.\\coreness} & \bigcell{c}{AVG.\\Corr.}\\ 
% 				\midrule
% 				\multirow{6}{*}{\shortstack{Edge-Dependent\\NodeLabel\\Prediction}} & Coauth-DBLP & 108,484 & 91,266 & 236 & 36 & .000,032 & 91,266 & 138,479 & 91,266 & 0.19 & 0.17 & 0.18 & 0.21 & 0.19\\ 
% 				& Coauth-AMiner & 1,712,433 & 2,037,605 & 752 & 115 & .000,001 & 2,037,605 & 1,652,332 & 1,503,061 & 0.23 & 0.22 & 0.22 & 0.30 & 0.24\\
% 				& Email-Enron & 21,251 & 101,124 & 18,168 & 948 & .000,552 & 635,268 & 450,129 & 101,124 & 0.09 & 0.09 & 0.05 & 0.18 & 0.10\\
% 				& Email-Eu & 986 & 209,508 & 8,659 & 59 & .002,623 & 209,508 & 332,334 & - & 0.24 & 0.22 & 0.32 & 0.25 & 0.24\\
% 				& Stack-Biology & 15,490 & 26,823 & 1,318 & 12 & .000,135 & 26,290 & 18,444 & 11,523 & 0.30 & 0.29 & 0.32 & 0.25 & 0.29\\
% 				& Stack-Physics & 80,936 & 200,811 & 6,332 & 48 & .000,030 & 194,575 & 201,121 & 84,113 & 0.31 & 0.31 & 0.33 & 0.26 & 0.30\\
% 				\midrule
% 				\multirow{3}{*}{\shortstack{DownStream\\Task}} & Ranking-Halo & 5,507 & 31,028 & 505 & 12 & .001,120 & \multicolumn{3}{c|}{} & \\
% 				& Return-Synthetic & 6,000 & 9,675 & 10 & 13 & .000,575 & 3,406 & 19,918 & 10,082 & \\
% 				& Clustering-DBLP & 2,123 & 1,000 & 22 & 25 & .001,829 & 997 & 1,885 & 1,000 & \\
% 				\bottomrule
% 			\end{tabular}}
% 	\end{center}
% 	%\vspace{-4mm}
% \end{table*}

\subsection{Dataset Detail}\label{appendix:data}
Table~\ref{tab:datasets} provides some statistics of the used datasets. In addition to elementary statistics, we also measure the degree of correlation between edge-dependent orders of node centralities and edge-dependent node labels. Specifically, we calculate the average of Cramer's coefficient matrix~\cite{cramer1946mathematical} between them. 
Related to Section~\ref{sec:evaluation:labeldist}, we report the average entropy in the label distribution of each node. Note that the average entropy is non-zero in all datasets, indicating that the labels of each node do vary in different hyperedges. 
In the co-authorship datasets, we exclude all publications where the order of authors are in alphabetical order since the such an order is likely to have no meaningful information.

\subsection{Node Centrality}\label{appendix:nodecentral}

For positional encoding, we leverage four node centrality values; degree, coreness~\cite{molloy2005cores, jiang2017parallel}, eigenvector centrality~\cite{bonacich1987power}, and PageRank~\cite{langville2005survey,page1999pagerank}. We define the degree of a node $v$ as $d(v) = |\{e \in \SE | v \in e \}|$. The k-core of a hypergraph is defined as the maximal sub-hypergraph where every node has at least degree $k$ within it. Then, the coreness of a node is defined as the maximum $k$ such that it belongs to the $k$-core. Eigenvector centrality and PageRank are calculated on a clique-expanded graph where the weight of each edge between nodes $u$ and $v$ is $w_{u, v} = |\{e \in \SE : v \in e \text{ and } u \in e \}|$. 
% We compute the coreness of each node by extending core decomposition algorithm~\cite{batagelj2003m} to hypergraphs. Formally, in hypergraph, a sub-hypergraph $\SGH = \{\SVH, \SEH = \{e \in \SE | v \in \SVH, \forall v \in e \}  \}$ is a k-core iff $\forall v \in \SVH : d_{\SGH}(v)* = |\{e \in \SEH | v \in e \}| \geq k $ and $\SGH$ is a maximum sub-hypergraph with this property. We use coreness of node $v$ as the highest order of a sub-hypergraph that contains this node.

\subsection{Parameter Setting}\label{appendix:hp}
The search spaces of hyperparameters are: 
\begin{itemize}[leftmargin=*]
    \item Learning rate: $\{0,001, 0.0001\}$.
    \item Number of layers: $\{1,2\}$ except for Coauthorship-AMiner, where we use one layer in HST, AST and \method.
    \item Size of batch: $\{64, 128\}$ except for Coauthorship-AMiner, where we use $\{256, 512\}$.
    \item Size of sample: $\{40, 100\}$. We sample incident hyperedges (but we do not sample but use all incident nodes) for efficiency with few exceptions: (a) all models in Coauthorship-DBLP, and HNHN, HGNN, HCHA, HAT, and (b) UniGCNII in StackOverflow-Biology.
    \item Hidden dimension: $64$.
    \item Dimension of final node and hyperedge embeddings: $128$.
    \item Dropout ratio: $0.7$.
    \item Number of the inducing points: $4$ (used in HST and \method).
    \item Number of attention layer: $2$ (used in HST and \method).
\end{itemize}
Exceptionally, for HCHA, we do not use sampling and train it in a full-batch setting. But we tune the hyperparameters of HCHA in larger search space: (1) learning rate $\in \{0.005, 0,01, 0.03, 0.05, 0.1\}$; (2) number of layers $\in \{1,2\}$; (3) dropout ratio $\in \{0.3, 0.5, 0.7\}$; (4) dimension of final node and hyperedge embedding $= 128$; (5) hidden dimension $=64$ (6) number of epochs $=300$ with early stopping.

% table for Choice of hyperparameters

\subsection{Additional Ablation Studies}

\smallsection{Positional Encoding}\label{appendix:abl_pe}
% Our model utilizes \PE as positional encoding. 
We study the usefulness of \PE by replacing it with other positional encoding schemes for graph neural networks (see Section~\ref{sec:pe}).
% exclude some positional encodings for baselines
% In our case, initial node features are generated by node2vec so nodes with similar neighbors have similar features. Because the input node features have already global positional information, we exclude using the random discriminating features, Weisfeiler-Lehman, Laplacian Eigenvector, and random-walk based positional encodings.
% relative positional encodings
% On the other hand, the relative positional encodings suit our intention of \PE. As \PE is the order of nodes by their centrality within a hyperedge, \PE provides the relative position of nodes. Therefore, we compare \PE with existing two relative positional encodings: Shaw et al.~\cite{shaw2018self} and GraphIT~\cite{mialon2021graphit}. To compute the distance between nodes, we apply two kinds of graph kernels, the diffusion kernel (DK) and p-step random walk kernel (PRWK) described in GraphIT.  
Since we generate initial node features using random-walk based embedding methods (see Section~\ref{sec:exp:setting}), global positional information is included in the node features to some degree. %Thus, \PE, which is the edge-dependent order of node centrality, gives additional information regarding each node's relative position in its hyperedge.
%In our case, the initial node features already include global positional information about nodes by node2vec, and our positional encoding gives the relative position of nodes by their centrality within hyperedges. 
Therefore we compare \PE with two relative positional encodings: Shaw et al.~\cite{shaw2018self} and GraphIT~\cite{mialon2021graphit}. 
For them, which require distances between nodes, we apply two kinds of graph kernels, the diffusion kernel (DK) and the p-step random walk kernel~\cite{mialon2021graphit} (PRWK), to them.
% To compute the distance between nodes, we apply two kinds of graph kernels, the diffusion kernel (DK) and p-step random walk kernel (PRWK) described in GraphIT.
% whole ranking
%Furthermore, we also experiment a variant of \PE: \textit{WholeOrderPE} 
In addition, in order to verify the importance of \textit{relativeness within hyperedge}, we use another positional encoding method named \textit{WholeOrderPE}. \textit{WholeOrderPE} is a variant of \PE which uses the global order of centrality among all nodes, instead of the relative order within each hyperedge.
% experiment - no inducing points
However, these relative positional encoding methods are hard to be used with inducing points. Thus, we do not use inducing points in this ablation study, and the base model is described as follows:
\begin{equation}\label{equation:abl_pe}
    \tilde{V}_{e}^{(l)} = MAB(V_{e}^{(l-1)}, V_{e}^{(l-1)} ; TypeOfPE)
\end{equation}
\begin{equation}
    H_e^{(l)} = \aggregation(\tilde{V}_{e}^{(l)}, H_e^{(l-1)})
\end{equation}
\begin{equation}
    X_v^{(l)} = \aggregation(\WithinAttention(E_{v}^{(l-1)}), X_v^{(l-1)})
\end{equation}
Thus, only Eq.~\eqref{equation:abl_pe} changes depending on positional encoding schemes. Since positional encoding schemes for hyperedge does not exist as far as we know, we do not use any positional encoding for message passing from hyperedges to nodes in this experiment. 
% Result
The result can be found in Table~\ref{tab:pe_ablation}. \PE  outperforms all other positional encoding methods.
%  The relative positional encoding based on Shaw et al. with diffusion kernel came out with the next good performance. 
The result of WholeOrderPE supports the effectiveness of using relative orders within hyperedges. 
% Additionally, \method w/o Inducing Points indicate the variant of \method without applying inducing points so that Equation~\ref{equation:method_att} is replaced by Equation~\ref{equation:abl_pe}. 
% The performances of these two models are comparable but we want to note that \method is more efficient.
For the fairness of comparison, we provide a variant of \method, \method w/o Inducing Points, which does not use inducing points.
%), since baseline positional encoding methods use all pair-node attention.
%as described in Eq~\ref{equation:abl_pe}. We call this variant as \method w/o Inducing Points. 
\method w/ and w/o Inducing Points always outperform other positional encodings. Note that these two methods showed competitive performances, while \method w/ Inducing Points is more efficient.

\smallsection{Advantage of \WithinAttention in both directions}\label{appendix:abl_partial}
Recall that we devise the \WithinAttention module for reflecting edge-dependent relationships between nodes within each hyperedge. But, we also use this module in the propagation from hyperedges to nodes. In order to confirm whether \WithinAttention is truly effective in both directions of message passings, we replace the message passing from hyperedges to nodes with the aggregation methods used in HNHN (\method + HNHN) and HAT (\method + HAT).
%we replaced the propagation at hyperedges with other modules. We experiment with HNHN and HAT, and each refers to \method + HNHN and \method + HAT. 
Table~\ref{tab:ablresult} shows that \method outperforms both \method + HNHN and \method + HAT. This justifies the use of the \WithinAttention module in both directions. Furthermore, it is also interesting to see that \method + HNHN and \method + HAT outperform vanilla HNHN and vanilla HAT, respectively.

% \smallsection{Reasonable Choice of \aggregation}\label{appendix:abl_agg}
% Because we can choose other architectures in \aggregation, we experiment two variants of our model arising from aggregating by average and aggregating by PMA defined in SetTransformer, which are denoted as \method w. AvgAgg and \method w. PMA respectively. As reported in Table~\ref{tab:ablresult}, our \method showed the highest performance on the Coauthorship-DBLP dataset. In StackOverflow-Biology dataset, \method is outperformed by aggregating by average. However, we believe that our \aggregation module is not worse because it is more expressive than aggregating by average and it has already proved a high performance on many datasets.

% ============================================================================================================================================
% \begin{table}[h]
%     \caption{Product Return Prediction}
%     \begin{center}
%         \scalebox{0.8}{
%         \begin{tabular}{l|c}
%         	\toprule
%         	Method & Precision\\
%         	\midrule
%         	Hypergraph w/ GroundTruth & \textbf{0.7553}\\
%         	\textbf{HyperGO w/ \method} & \underline{0.7536} \\
%         	HyperGo w/o Labels &  0.7526 \\ 
%         	\bottomrule
%         \end{tabular}}
%     \end{center}
% \end{table}

\subsection{Detailed Description of Downstream Tasks for \method}\label{appendix:downstream}
\smallsection{Ranking Aggregation} % --------------------------------------------------------------------------------------------------------------

\noindent\textbf{Data.} We use the Halo 2 game dataset as described in ~\cite{chitra2019random}. The Halo 2 game dataset consists of 5,507 users and two kinds of matches: 31,028 free-for-all matches where up to 8 players can involve in a game, and 5,093 1-v-1 matches where two members play the game.
% The free-for-all matches where up to 8 players play together are used for estimating the overall rankings of players. The 1-v-1 matches where only two players compete are used to evaluate how accurately each method predicts the winner. 
We use free-for-all matches to train and evaluate an edge-dependent node label classifier, and 1-v-1 matches as the test data for the downstream task.
We build a hypergraph by regarding players as nodes and matches as hyperedges.
% Players and matches are taken as nodes and hyperedges when modeling data into a hypergraph. 
The players are classified into their contribution levels during each match.
\noindent\textbf{Training.}
The continuous scores that the users get in each match are binned, and we use the binning index to indicate the contribution level of each player in the match, i.e., edge-dependent node labels. 
In detail, we normalize the scores during each match and divide the normalized scores into five bins containing 1/5 (20\%) of the scores. 
We train our model with free-for-all matches by splitting them into train/valid/test sets and predict all edge-dependent node labels in free-for-all matches. 
On the hypergraphs with predicted edge-dependent node labels, the overall rankings of players are estimated by the stationary distribution of the random walks as proposed in~\cite{chitra2019random}.
During the random walks, the node with a higher contribution level is visited more frequently within the hyperedge. In the evaluation on the 1-v-1 matches, we predict the winner as the one with the highest stationary probability. 
\noindent\textbf{Results.} 
We compare the method with four competitors described in ~\cite{chitra2019random}: (a) ranking aggregation based on random walks on a hypergraph with ground-truth scores, (b) that on a clique-expanded graph, and (c) a Markov chain-based ranking aggregation~\cite{dwork2001rank}, which is called MC3, and TrueSkill, which is developed by Microsoft~\cite{herbrich2006trueskill}. 
Additionally, we analyze the improvement from a hypergraph without edge-dependent node labels (i.e., without match scores).
% which tells just which players played together.
The method based on \method is second-best among the competitors. Surprisingly, it even slightly outperforms that of a hypergraph with ground-truth scores, which shows that  binning could lead to a better performance. 
%Our performance is quite comparable to TrueSkill, and 8.3\% of 1-v-1 matches are correctly predicted by our model, whereas those missed by TrueSkill. 

\smallsection{Clustering}\label{sec:eval_downstream_clustering}  % --------------------------------------------------------------------------------------------------------------

\noindent\textbf{Data.} We used the data extracted from  Coauthorship-DBLP where authors and publications are nodes and hyperedges, respectively. Following the dataset description~\cite{Swati2016dblp}, we select hyperedges that belong to only one category among computer science, data engineering, software engineering, and theory. 
Then, we choose a set of hyperedges among them that compose one connected component. 
% The extracted data consists of 33,050 hyperedges (publications) and 52,560 nodes (authors). 
In this data, edge-dependent node labels represent the orders of authors in each publication, and three categories are used, as described in Section~\ref{benchmark_dataset}.
\textbf{Training.} We train \method to predict the order of authors in each publication. After predicting the orders of all authors in each publication, we assign two as weights to the first and last authors and one to the others, as in \cite{chitra2019random}. 
% \begin{equation*}\label{equation:nodeweight_clustering}
%     \gamma_{e}(v) = \begin{cases}
%  2 & \text{ if the vertex } v \text{ is the first or last author of publication} \\
%  1 & \text{ if the vertex } v \text{ is a middle author of publication}
% \end{cases}
% \end{equation*}
Then we apply the clustering algorithm (RDC-Spec) proposed in ~\cite{hayashi2020hypergraph}. Specifically, the stationary distribution of random walks, which proceed in consideration of node weights, is used for spectral clustering.
\textbf{Results.} We compare the performance of RDC-Spec on three different hypergraphs, which are with ground-truth, predicted, and no labels, respectively. %The way to weigh according to the author's position is the same as above. 
The performance with labels predicted by \method is better than that with no labels, while that with ground-truth labels is best. Thus, predicting the orders of authors in each publication (i.e., edge-dependent node labels) is beneficial in hypergraph clustering.

\smallsection{Product Return Prediction}  % --------------------------------------------------------------------------------------------------------------

\noindent\textbf{Data.} We use a synthetic dataset from ~\cite{li2018tail} for the product return prediction task. It consists of 6,000 baskets and 10,000 products, which are nodes and hyperedges, respectively. 
The return rate of each product is assigned by the truncated normal distribution with mean 0.5 and standard deviation 1.0. The count of products in each basket is from 1 to 3 with the probabilities 60\%, 30\%, and 10\%. The baskets are labeled based on the count of products in them.
\textbf{Training.} We directly use the count of products in each basket as edge-dependent node labels and train \method to predict them. We then run HyperGo~\cite{li2018tail} on the hypergraph with predicted counts.
\textbf{Results.} As in the previous tasks, we compare the result of HyperGo on three different hypergraphs, which are with ground-truth, predicted, and no counts of products in each basket. The hypergraph with unknown counts indicates a situation in which you only know if the product is in a basket without knowing if there are duplicates or not. The method with the labels predicted by \method was second best, outperforming that without labels. %and the result after the case of the ground-truth in this downstream task. 
This result demonstrates the usefulness of identifying edge-dependent node labels in the considered application.
%also supports the usefulness of identifying edge-dependent node labels by \method in real-life.


% ==========================================================================================================================================
% \subsection{Details of Baselines}\label{appendix:baseline}
% HGNN updates node embeddings from neighbor nodes without explicitly obtaining hyperedge embeddings. To be specific, the node embedding is updated as follows,
% \begin{equation*}
%     X_v^{(l+1)} = \sigma(\frac{1}{\sqrt{d_v}} \sum_{e:v \in e} \frac{w_e}{|e|} \sum_{u:u \in e} \frac{X_u^{(l)}W^{(l)}}{\sqrt{d_u}})
% \end{equation*}
% where $X_v^{(l)}$ denotes the embedding of the node $v$ at the $l$-th layer, $d_v$ indicates the degree of node $v$, $w_e$ is a weight of hyperedge $e$ and $W^{(l)}$ is the weight matrix in the $l$-th layer.
% We devide this propagation as two steps to regard the intermediate output $Z_e$ as the embedding of the hyperedge $e$.
% \begin{equation*}
%     Z_e^{(l+1)} = \sum_{u:u \in e} \frac{X_u^{(l)}W^{(l)}}{\sqrt{d_u}}
% \end{equation*}
% \begin{equation*}
%     X_v^{(l+1)} = \sigma(\frac{1}{\sqrt{d_v}} \sum_{e:v \in e} \frac{w_e}{|e|} Z_e^{(l+1)})
% \end{equation*}

% Similar to this propagation, HCHA updates node embeddings as follows,
% \begin{equation*}
%     X_v^{(l+1)} = \sigma(\frac{1}{\sqrt{d_v}} \sum_{e:v \in e} \frac{w_e \alpha_{ve} ^{(l)}}{|e|} \sum_{u:u \in e} \frac{\alpha_{ue}^{(l)} X_u^{(l)}W^{(l)}}{\sqrt{d_u}})
% \end{equation*}
% where $\alpha_{ue}^{(l)}$ denotes the attention weight between the node $u$ and the hyperedge $e$. The attention weight is defined in HCHA,
% \begin{equation*}
%     \alpha_{ue}^{(l)} = \frac{exp(\sigma(a^{T}[X_u^{(l)} || Z_e^{(l)}])) }{\sum_{e':u \in e'} exp(\sigma(a^{T}[X_u^{(l)} || Z_e'^{(l)}])) }
% \end{equation*}
% As above, we also devide this process as follows,
% \begin{equation*}
%     Z_e^{(l+1)} = \sum_{u:u \in e} \frac{\alpha_{ue}^{(l)} X_u^{(l)}W^{(l)}}{\sqrt{d_u}}
% \end{equation*}
% \begin{equation*}
%     X_v^{(l+1)} = \sigma(\frac{1}{\sqrt{d_v}} \sum_{e:v \in e} \frac{w_e \alpha_{ve}^{(l)}}{|e|} Z_e^{(l+1)})
% \end{equation*}

% Since HCHA uses the same attention weight between the node and the hyperedge when updating in two steps, we designed HAT which separated the attention weight.
% In propagation from nodes to hyperedges, the hyperedge embedding is updated as follows,
% \begin{equation*}
%     Z_e^{(l+1)} = \sum_{u:u \in e} \alpha_{ue}^{(l)} X_u^{(l)}W^{(l)}
% \end{equation*}
% where attention is defined as,
% \begin{equation*}
%     \alpha_{ue}^{(l)} = \frac{exp(\frac{\sigma( Q_e^{T}K_u)}{\sqrt{d_k}})}{\sum_{u':u \in e} exp(\frac{\sigma( Q_e^{T}K_{u'})}{\sqrt{d_k}}) }
% \end{equation*}
% where the query vector $Q_e = Z_e^{(l)} W_q^{(l)}$ and the key vector $K_u = X_u^{(l)} W_k^{(l)}$. The $d_k$ denotes the dimension of key vector.

% In propagation from hyperedges to nodes, the node embedding is updated as follows,
% \begin{equation*}
%     X_v^{(l+1)} = \sigma( \sum_{e:v \in e} \hat{\alpha}_{ve}^{(l)} Z_e^{(l+1)})
% \end{equation*}
% where the attention is defined as,
% \begin{equation*}
%     \hat{\alpha}_{ve}^{(l)} = \frac{exp(\frac{\sigma( Q_v^{T}K_e)}{\sqrt{d_k}})}{\sum_{e':v \in e} exp(\frac{\sigma( Q_v^{T}K_{e'})}{\sqrt{\hat{d_k}}}) }
% \end{equation*}
% where the query vector $Q_v = X_v^{(l)} \hat{W_q}^{(l)}$ and the key vector $K_e = Z_e^{(l)} \hat{W_k}^{(l)}$. The $\hat{d_k}$ denotes the dimension of key vector.
